# Supplementary material for: Post-Selection Confidence Bounds for Prediction Performance
Source: arXiv:2210.13206 ancillary file (2023-02-03)
Supplement: Supplementary file 1 [file supplement.pdf]

# SUPPLEMENTARY INFORMATION TO POST-SELECTION CONFIDENCE BOUNDS FOR PREDICTION PERFORMANCE

**Pascal Rink**[*]
Center for Industrial Mathematics and
Competence Center for
Clinical Trials Bremen
University of Bremen
Bremen, Germany

**Werner Brannath**
Institute for Statistics and
Competence Center for
Clinical Trials Bremen
University of Bremen
Bremen, Germany

November 11, 2022

In this Supplementary Information, we present all the results of our simulation experiments in detail in order to assess the goodness of our proposed multiplicity-adjusted bootstrap tilting confidence bounds in comparison to all the considered standard approaches. For details, see Section 3, where we only presented selected results of our simulation experiments. These are the main arguments why we dismiss some and highlight others there:

1. As to the preselection of models, the gain of cross-validation over the simple max-approach is small in both the size of the lower confidence bound as well as true model performance. However, cross-validation is the more stable approach and the competing methods are harder to compete with for our proposed confidence bounds.
2. The Wald normal approximation confidence bound is too liberal for small sample sizes and reaches the nominal coverage probability in our experiments only in the case where multiple models are preselected and the Šidák correction is employed. Therefore we cannot recommend Wald bounds as a universal approach.
3. In case of preselection of multiple models, the Šidák-corrected versions of the Wilson and Clopper-Pearson confidence bounds are more conservative than the unadjusted versions. This conservatism outweights the gain in both true model performance and size of the lower confidence bound, induced by the gainful multiple selection, and thus the Šidák-correction versions are inferior to their unadjusted versions in the default pipeline.
4. The same applies to the Šidák-corrected version of the DeLong and Hanley-McNeil bounds for the AUC.
5. The results for the Hanley-McNeil and the DeLong approach for the AUC are similar, so we only present the DeLong results since they seem to be more widely used.
6. In comparison to the Wilson bounds, the Clopper-Pearson bounds are smaller and more conservative.
7. The within 1 standard error and the top 10 % selection rules yield similar results. However, since the present multiplicity is usually stronger in case of the top 10 % selection rule, we only present those results here because this renders our conclusions more defensive.

The following pages present the remaining results. There is a separate section for each configuration of simulation parameters. As in the main document we compare the confidence interval methods in terms of four aspects: coverage probability, size of lower confidence bound, true performance of the final selected model, and *tightness* of the lower confidence bound, which is the distance between the true performance and the lower bound.

[*]Correspondence to: Pascal Rink, p.rink@uni-bremen.de

# 1 Prediction Accuracy, Case A Features, Sample Size 200, With Cross-Validation

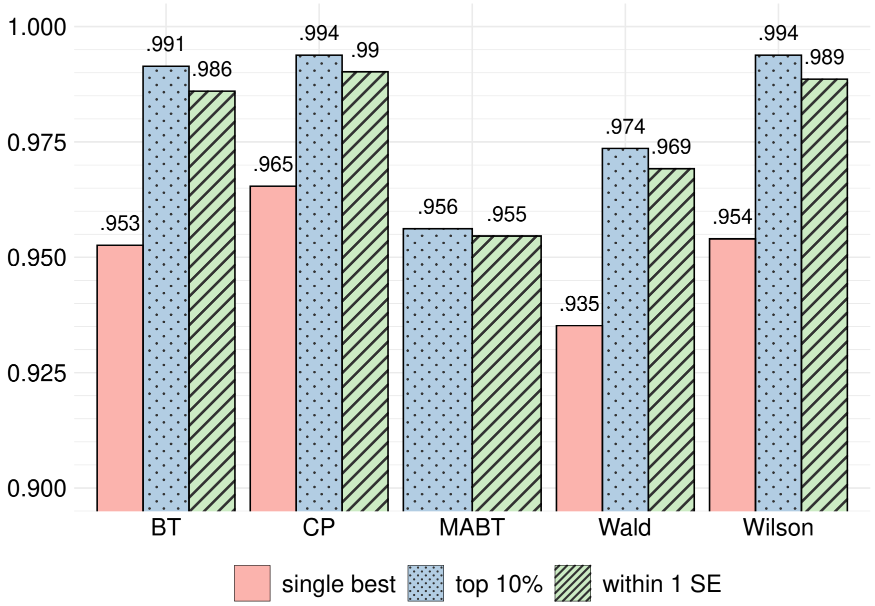


Figure 1: Observed coverage for prediction accuracy with case A features, learning sample size 150, evaluation sample size 50, and with cross-validation for validation performance estimation. MABT coverage is close to the nominal level and only slightly conservative, as are BT and Wilson bounds from using the *single best* selection rule. All the Šidák-corrected bounds are heavily conservative. Wald bounds using the *single best* selection rule are too liberal

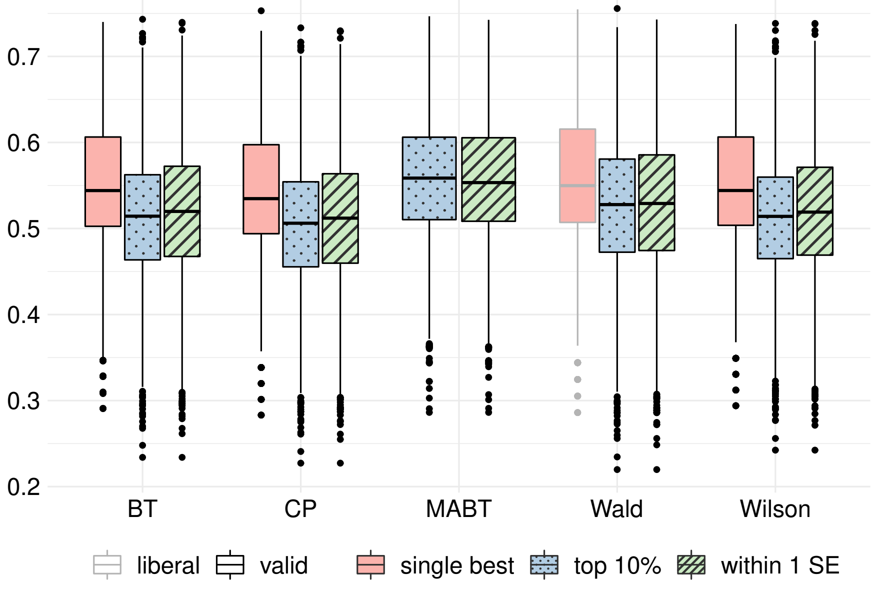


Figure 2: Lower confidence bounds for prediction accuracy with case A features, learning sample size 150, evaluation sample size 50, and with cross-validation for validation performance estimation. MABT bounds are the largest. The bounds from the *single best* selection rule are slightly smaller, while all the Šidák-corrected bounds are clearly smaller than MABT bounds

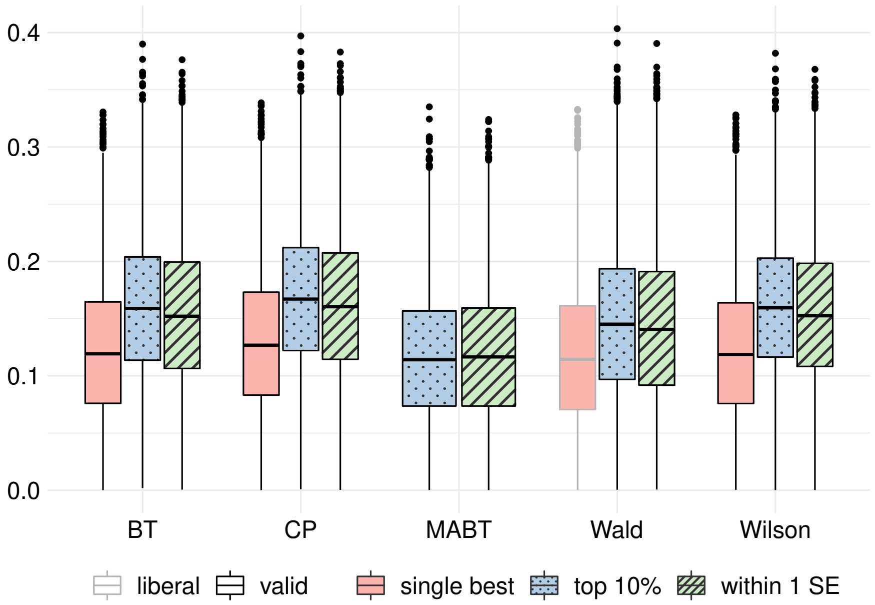


Figure 3: Tightness for prediction accuracy with case A features, learning sample size 150, evaluation sample size 50, and with cross-validation for validation performance estimation. MABT bounds are the tightest. The bounds from the *single best* selection rule are slightly less tight, while all the Šidák-corrected bounds are clearly less tight than MABT bounds

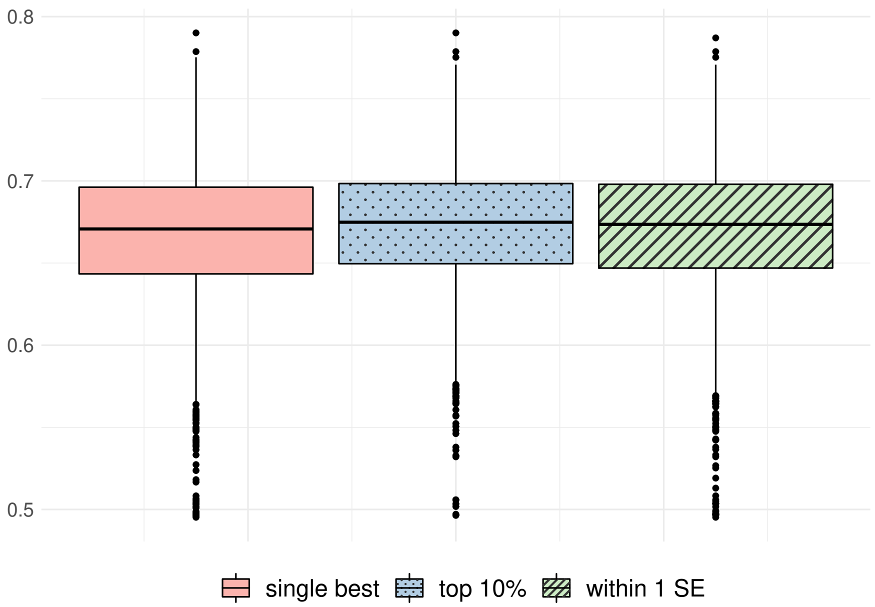


Figure 4: True prediction accuracy of the final selected model with case A features, learning sample size 150, evaluation sample size 50, and with cross-validation for validation performance estimation. The true prediction accuracies from the *top 10%* and *within 1 SE* selection rules are both slightly higher than from the *single best* selection rule

## 2 Prediction Accuracy, Case A Features, Sample Size 200, Without Cross-Validation

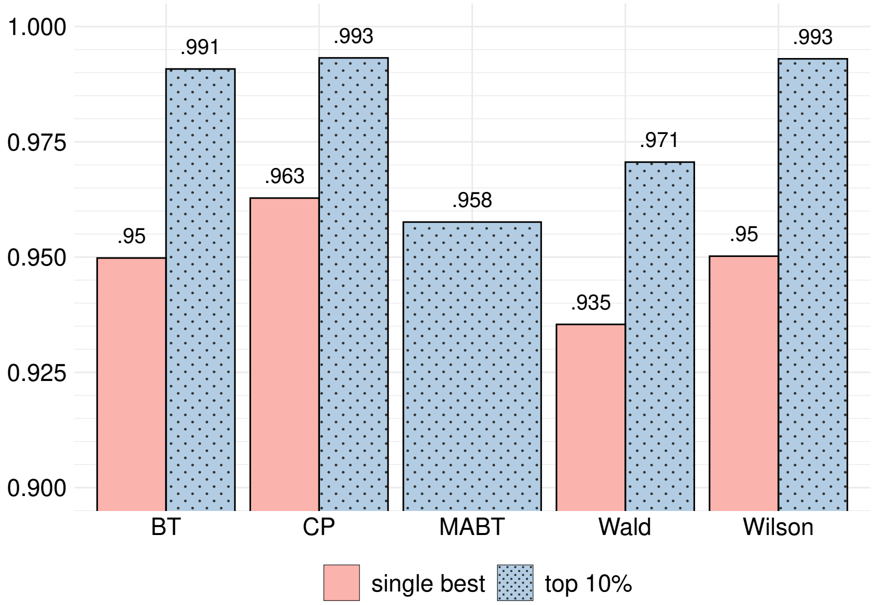


Figure 5: Observed coverage for prediction accuracy with case A features, learning sample size 150, evaluation sample size 50, and without cross-validation for validation performance estimation. BT and Wilson bounds from the *single best* selection rule have nominal coverage, while MABT bounds are slightly conservative, CP bounds even a little more. All the Šidák-corrected bounds are strongly conservative

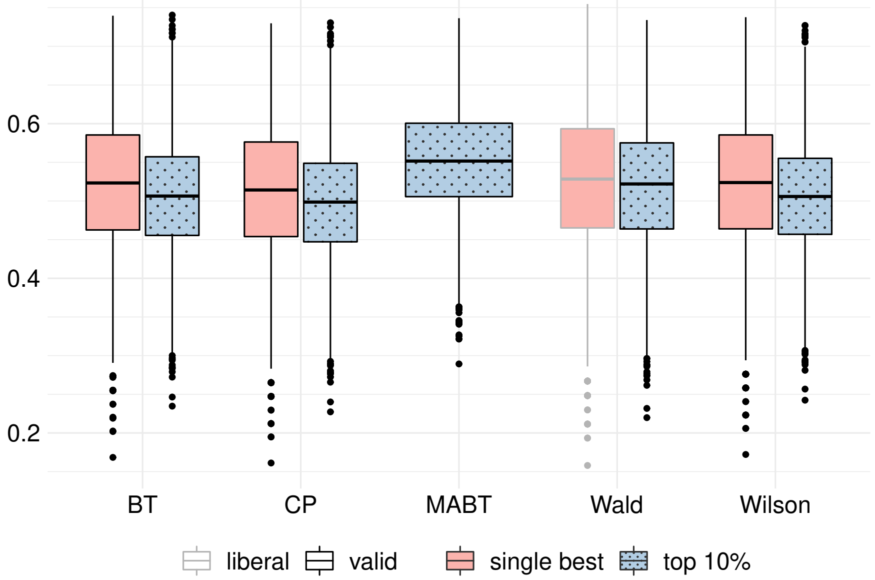


Figure 6: Lower confidence bounds for prediction accuracy with case A features, learning sample size 150, evaluation sample size 50, and without cross-validation for validation performance estimation. MABT bounds are the largest. The bounds from the *single best* selection rule are visibly smaller than MABT, and the Šidák-corrected bounds are even a bit smaller

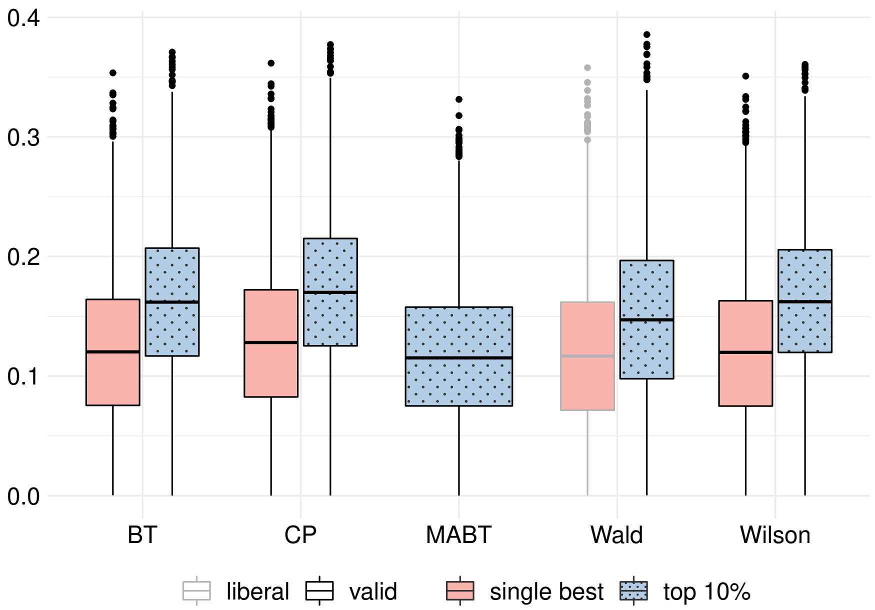


Figure 7: Tightness for prediction accuracy with case A features, learning sample size 150, evaluation sample size 50, and without cross-validation for validation performance estimation. MABT bounds are the tightest. The bounds from the *single best* selection rule are a bit less tight, and all the Šidák-corrected bounds are even less tight

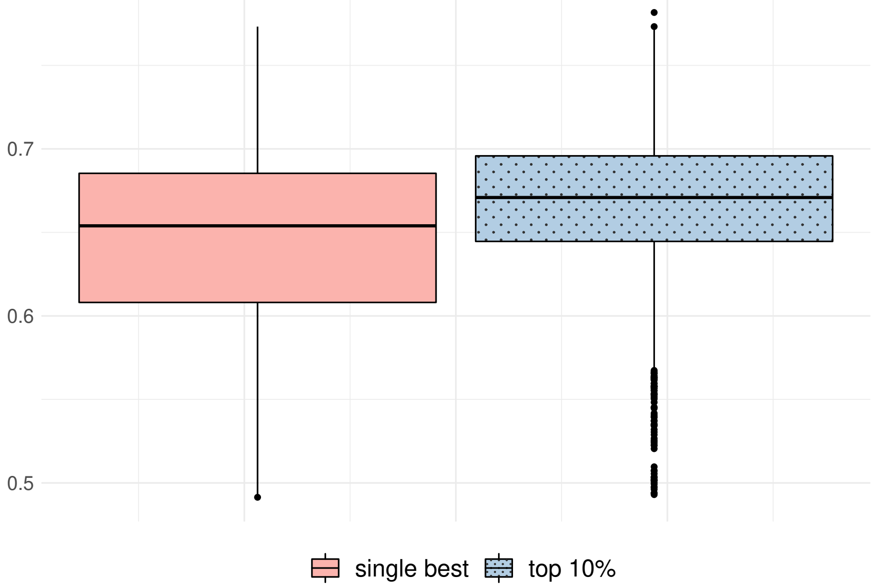


Figure 8: True prediction accuracy of the final selected model with case A features, learning sample size 150, evaluation sample size 50, and without cross-validation for validation performance estimation. The true prediction accuracies from the *top 10%* selection rule are visibly higher than from the *single best* selection rule

## 3 Prediction Accuracy, Case A Features, Sample Size 400, With Cross-Validation

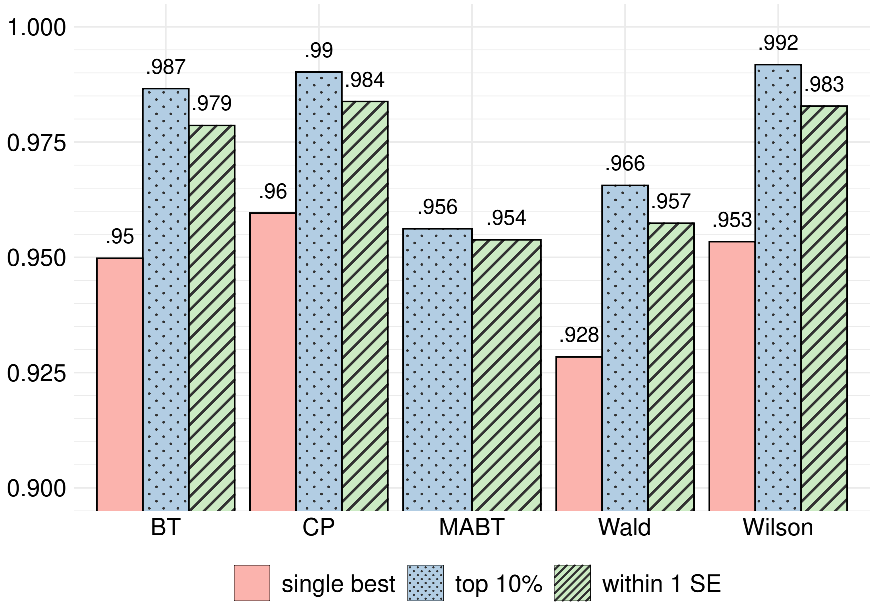


Figure 9: Observed coverage for prediction accuracy with case A features, learning sample size 300, evaluation sample size 100, and with cross-validation for validation performance estimation. MABT bounds are slightly conservative, as are Wilson and CP bounds from the *single best* selection rule. BT bounds have the nominal coverage. Wald bounds from the *single best* selection rule are clearly too liberal. All the Šidák-corrected bounds are heavily conservative

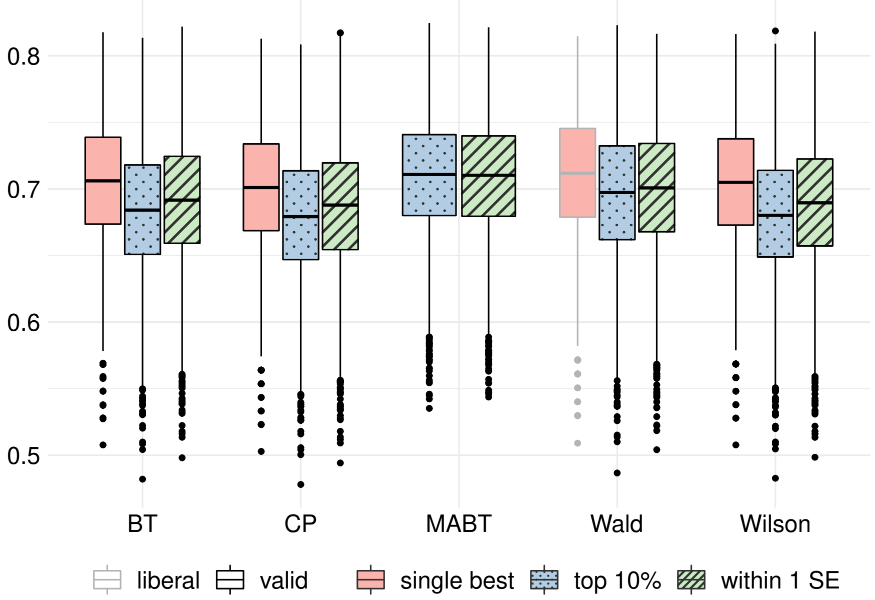


Figure 10: Lower confidence bounds for prediction accuracy with case A features, learning sample size 300, evaluation sample size 100, and with cross-validation for validation performance estimation. MABT bounds are the largest. The bounds from the *single best* selection rule are slightly smaller, and all the Šidák-corrected bounds are even smaller

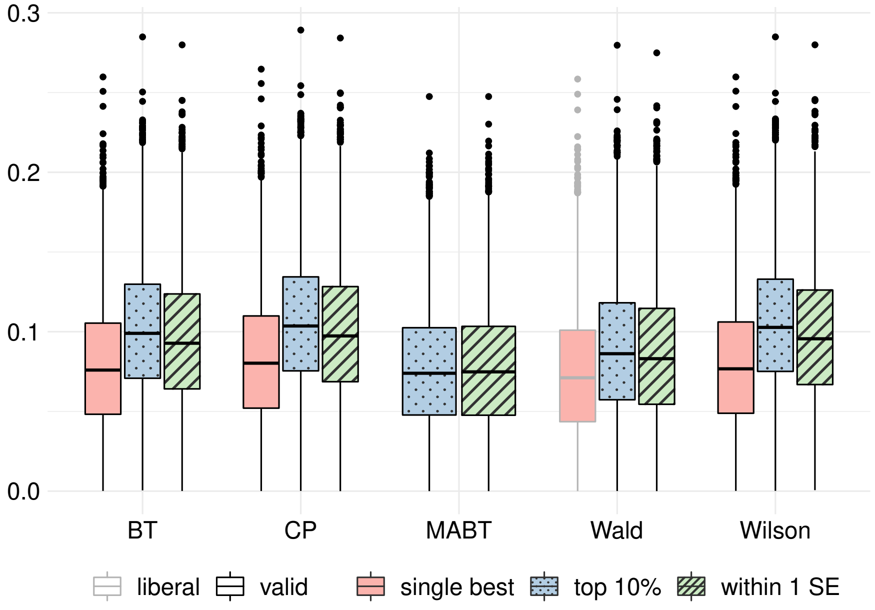


Figure 11: Tightness for prediction accuracy with case A features, learning sample size 300, evaluation sample size 100, and with cross-validation for validation performance estimation. MABT bounds are the tightest. The bounds from the *single best* selection rule are a bit less tight, and all the Šidák-corrected bounds are even less tight than those

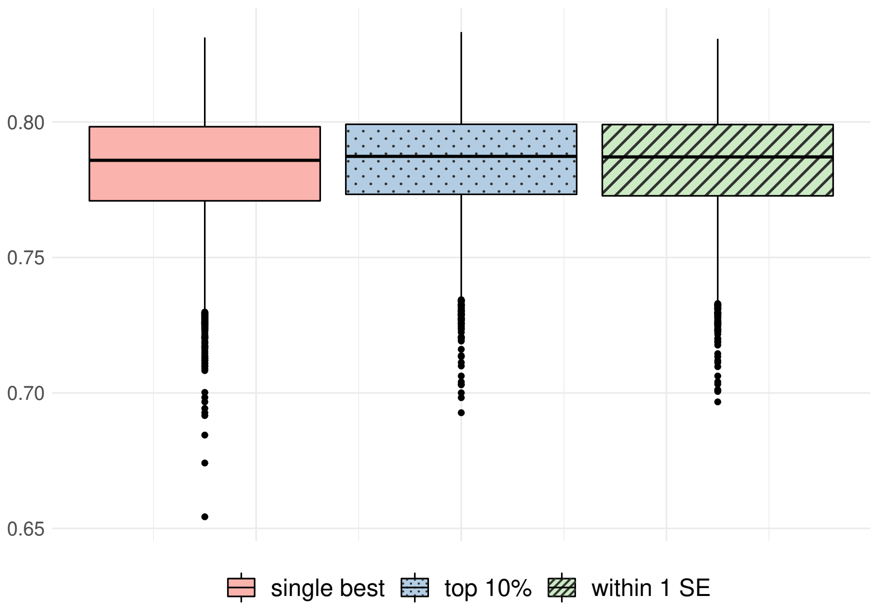


Figure 12: True prediction accuracy of the final selected model with case A features, learning sample size 300, evaluation sample size 100, and with cross-validation for validation performance estimation. The true prediction accuracies from the *top 10%* and *within 1 SE* selection rules are both higher than from the *single best* selection rule

# 4 Prediction Accuracy, Case A Features, Sample Size 400, Without Cross-Validation

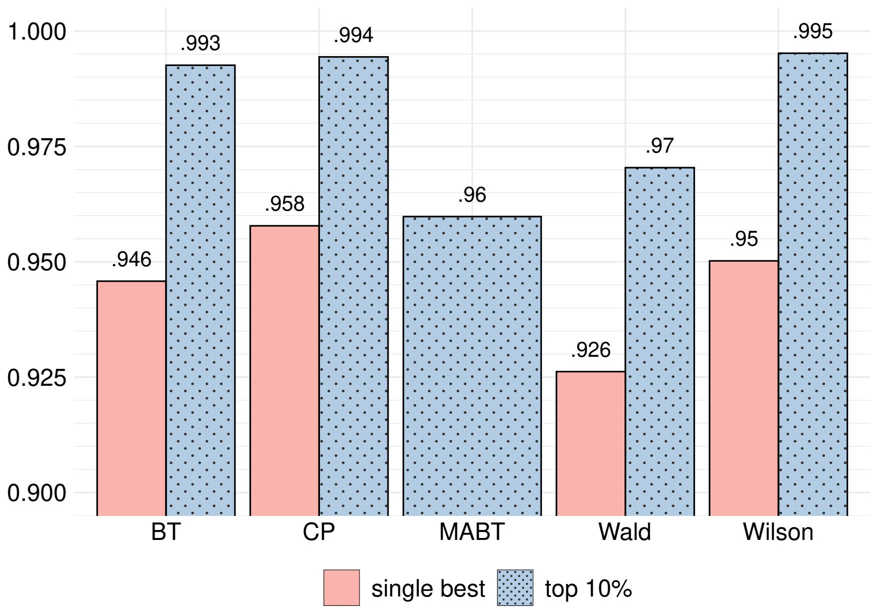


Figure 13: Observed coverage for prediction accuracy with case A features, learning sample size 300, evaluation sample size 100, and without cross-validation for validation performance estimation. From the *single best* selection rule, CP bounds are slightly conservative, Wilson bounds have the nominal coverage, BT bounds are slightly liberal, and Wald bounds are very liberal. All the Šidák-corrected bounds are very conservative

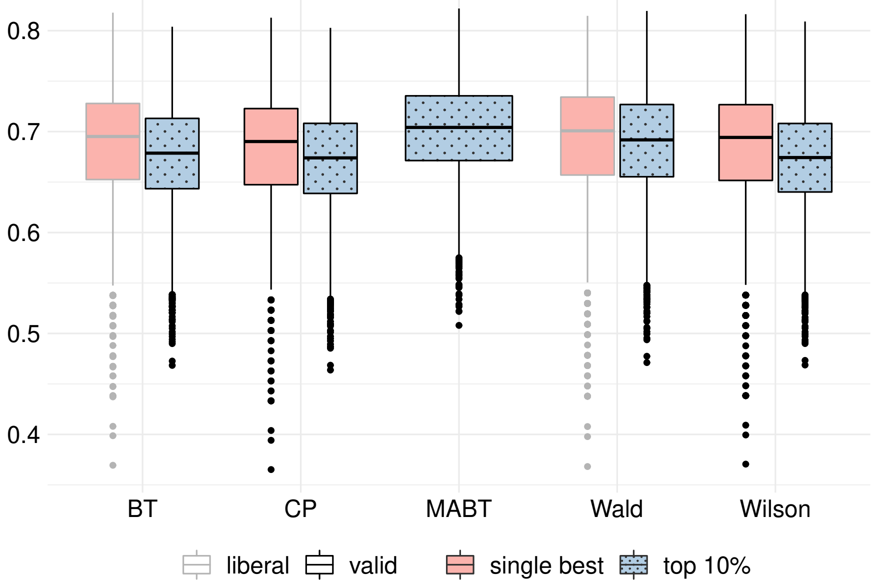


Figure 14: Lower confidence bounds for prediction accuracy with case A features, learning sample size 300, evaluation sample size 100, and without cross-validation for validation performance estimation. MABT bounds are the largest. CP and Wilson bounds from the *single best* selection rule are only slightly smaller, and all the Šidák-corrected bounds are even smaller

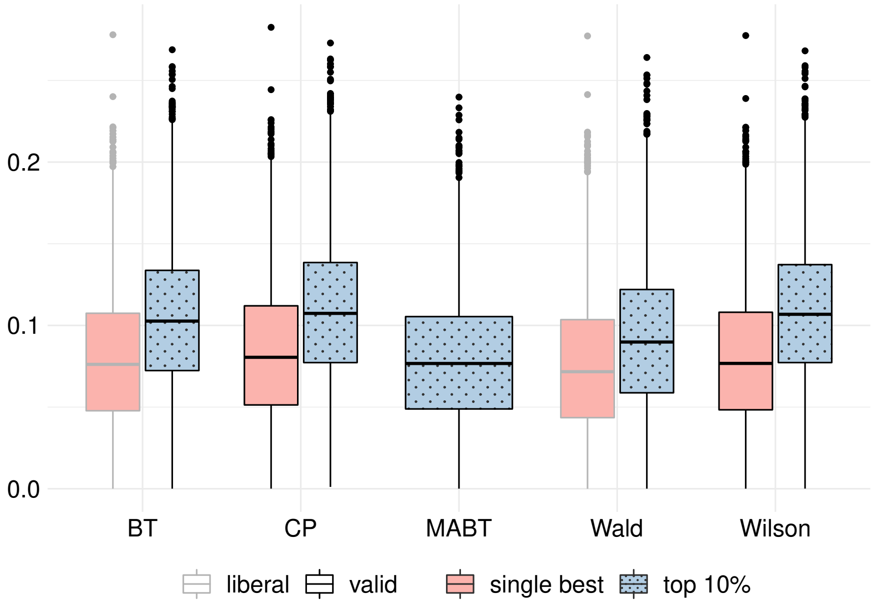


Figure 15: Tightness for prediction accuracy with case A features, learning sample size 300, evaluation sample size 100, and without cross-validation for validation performance estimation. MABT bounds are the tightest among those reaching the nominal level. CP and Wilson bounds from the *single best* selection rule are slightly less tight, and all the Šidák-corrected bounds are even less tight than those

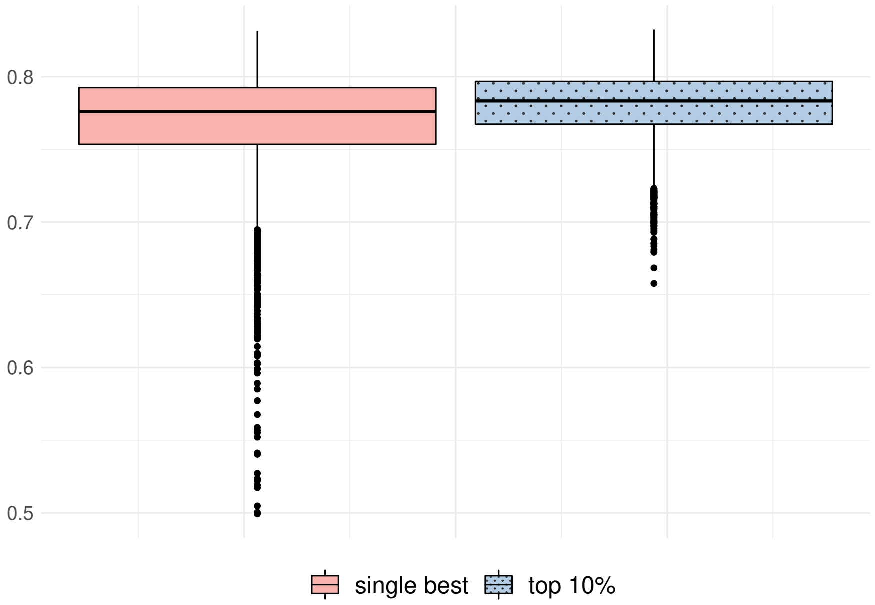


Figure 16: True prediction accuracy of the final selected model with case A features, learning sample size 300, evaluation sample size 100, and without cross-validation for validation performance estimation. The true prediction accuracies from the *top 10%* selection rule are visibly higher than from the *single best* selection rule

## 5 Prediction Accuracy, Case B Features, Sample Size 200, With Cross-Validation

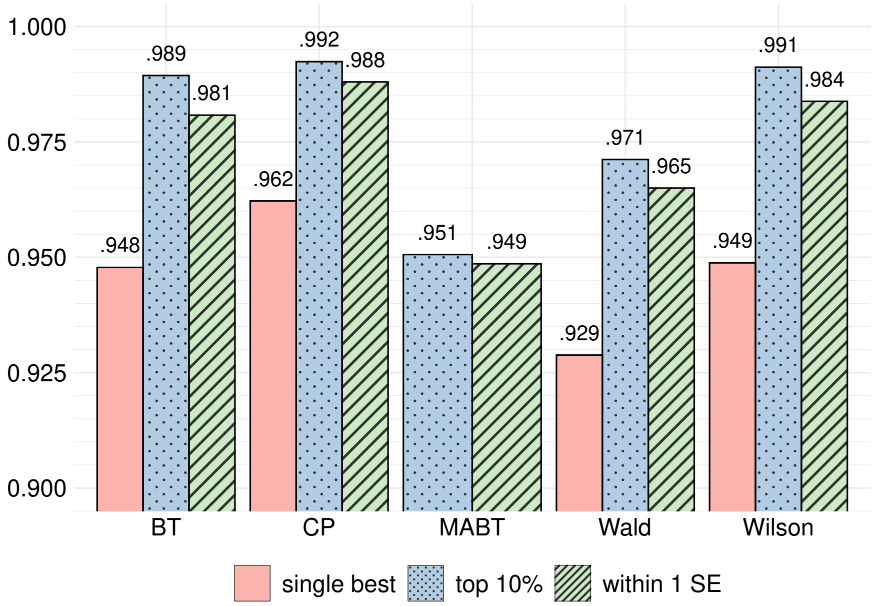


Figure 17: Observed coverage for prediction accuracy with case B features, learning sample size 150, evaluation sample size 50, and with cross-validation for validation performance estimation. MABT bounds are very close to the nominal level, as are BT and Wilson bounds from the *single best* selection rule. Wald bounds from the *single best* selection rule are very liberal, while all the Šidák-corrected bounds are very conservative

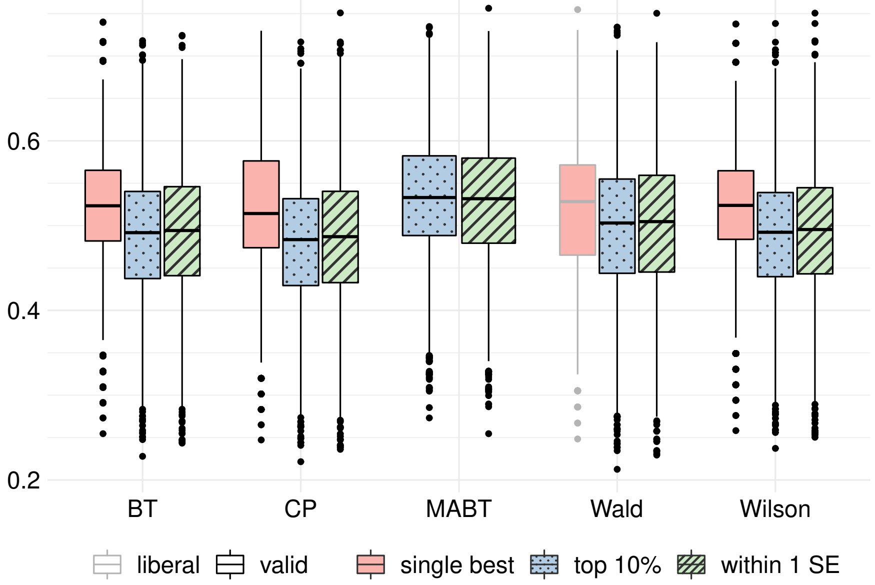


Figure 18: Lower confidence bounds for prediction accuracy with case B features, learning sample size 150, evaluation sample size 50, and with cross-validation for validation performance estimation. MABT bounds are the largest. The bounds from the *single best* selection rule are a bit smaller, and the Šidák-corrected bounds are even smaller than those

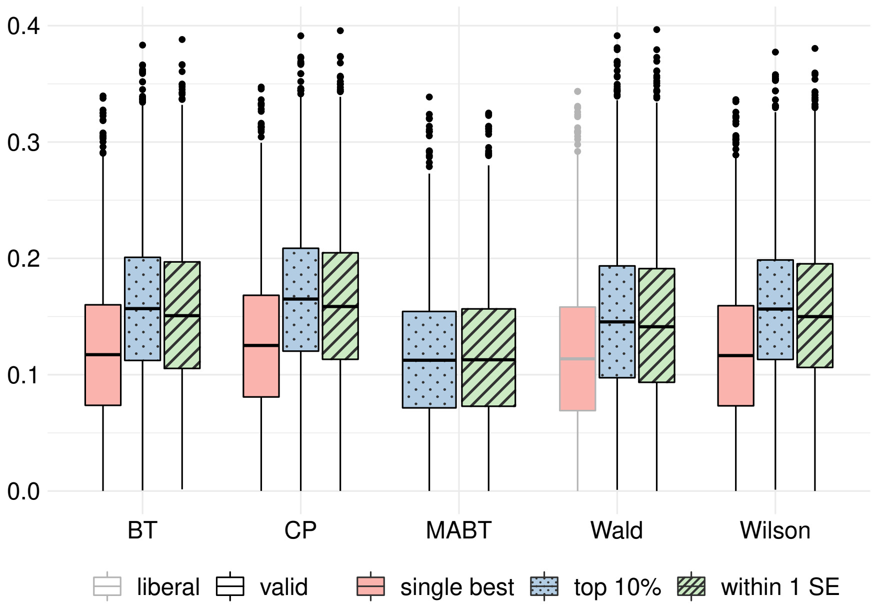


Figure 19: Tightness for prediction accuracy with case B features, learning sample size 150, evaluation sample size 50, and with cross-validation for validation performance estimation. MABT bounds are tightest. The bounds from the *single best* selection rule are less tight, and the Šidák-corrected bounds are even less tight than those

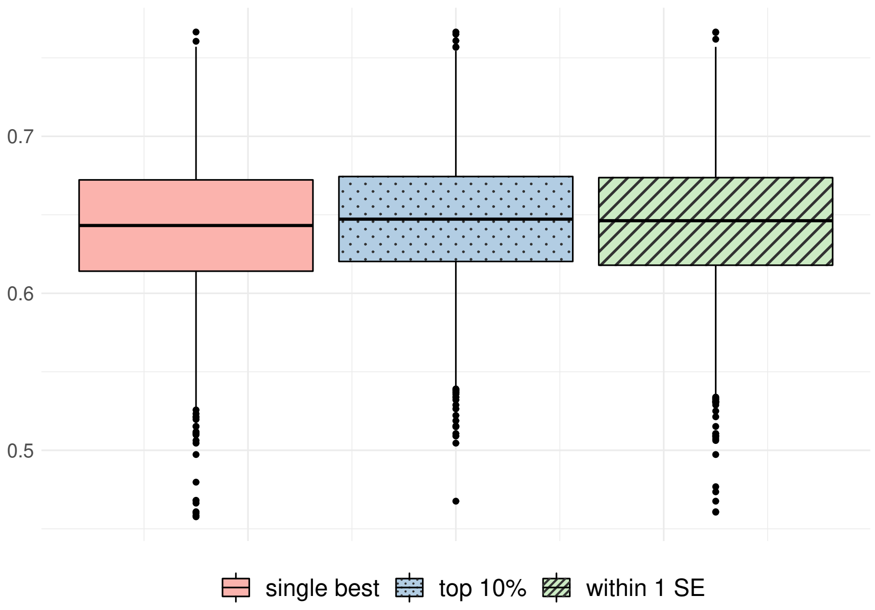


Figure 20: True prediction accuracy of the final selected model with case B features, learning sample size 150, evaluation sample size 50, and with cross-validation for validation performance estimation. The true prediction accuracies from the *top 10%* and *within 1 SE* selection rules are both higher than from the *single best* selection rule

# 6 Prediction Accuracy, Case B Features, Sample Size 200, Without Cross-Validation

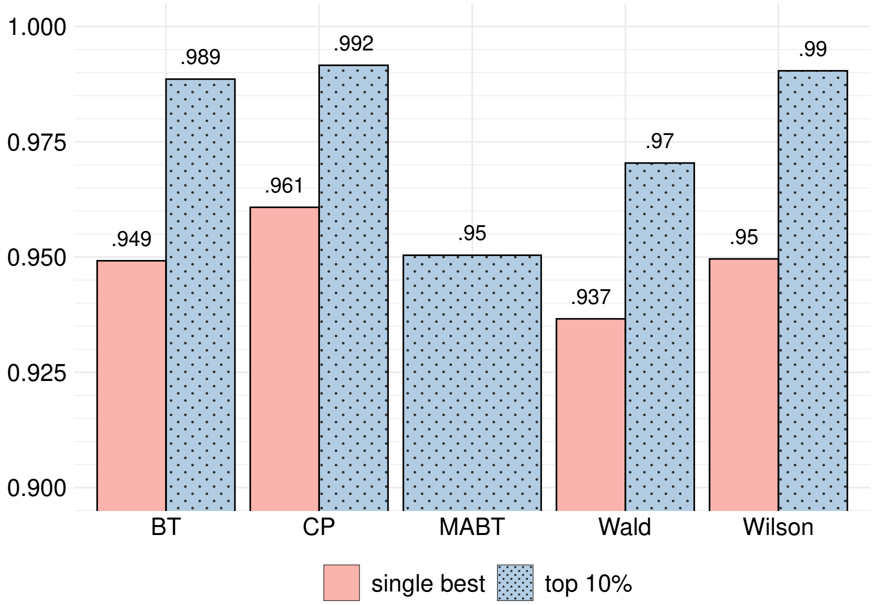


Figure 21: Observed coverage for prediction accuracy with case B features, learning sample size 150, evaluation sample size 50, and without cross-validation for validation performance estimation. Wilson bounds from the *single best* selection rule and MABT bounds have the nominal level, while BT is very close to it. Using the *single best* selection rule, CP is conservative, while Wald is too liberal. All the Šidák-corrected bounds are heavily conservative

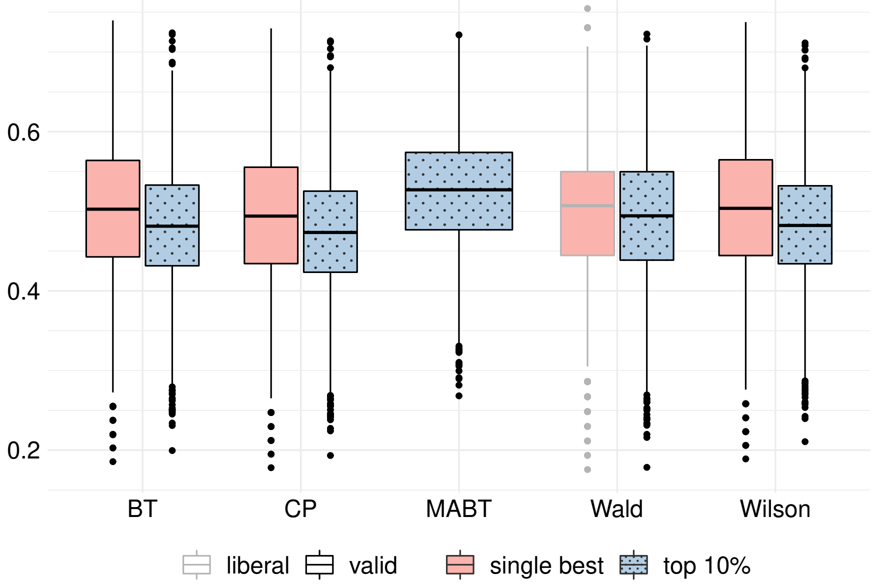


Figure 22: Lower confidence bounds for prediction accuracy with case B features, learning sample size 150, evaluation sample size 50, and without cross-validation for validation performance estimation. MABT bounds are largest. The bounds from the *single best* selection rule are smaller, and the Šidák-corrected bounds are even smaller than those

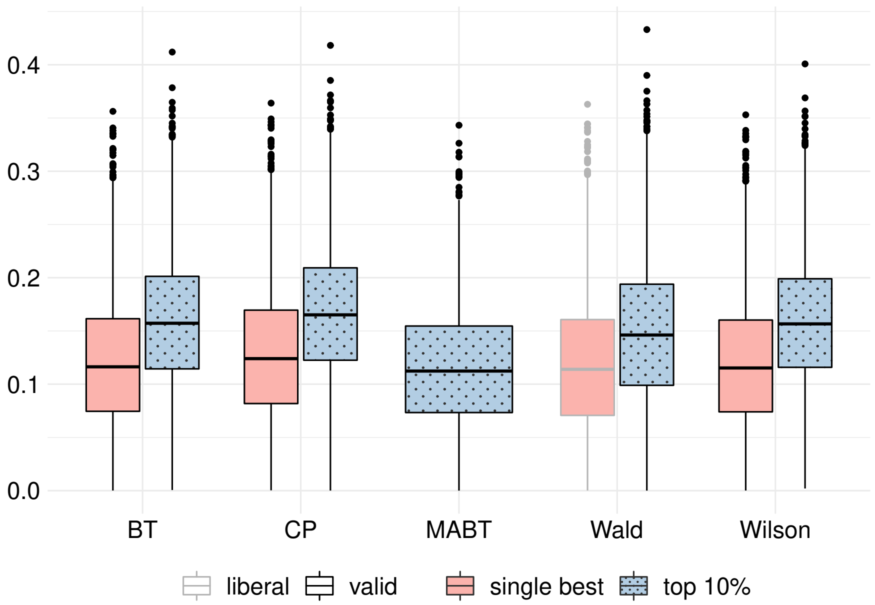


Figure 23: Tightness for prediction accuracy with case B features, learning sample size 150, evaluation sample size 50, and without cross-validation for validation performance estimation. MABT bounds are tightest. The bounds from the *single best* selection rule are slightly less tight, and the Šidák-corrected bounds are clearly even less tight

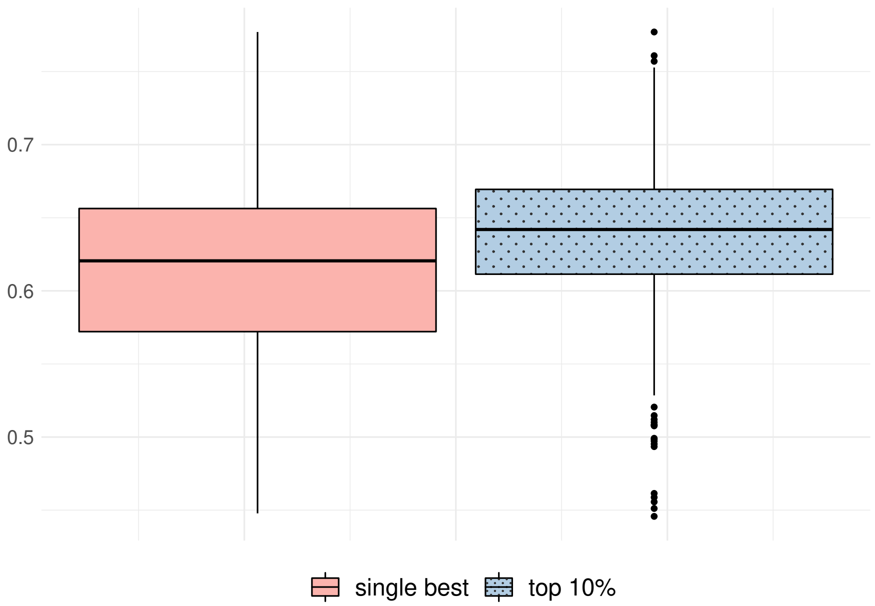


Figure 24: True prediction accuracy of the final selected model with case B features, learning sample size 150, evaluation sample size 50, and without cross-validation for validation performance estimation. The true prediction accuracies from the *top 10%* selection rule are clearly higher than from the *single best* selection rule

# 7 Prediction Accuracy, Case B Features, Sample Size 400, With Cross-Validation

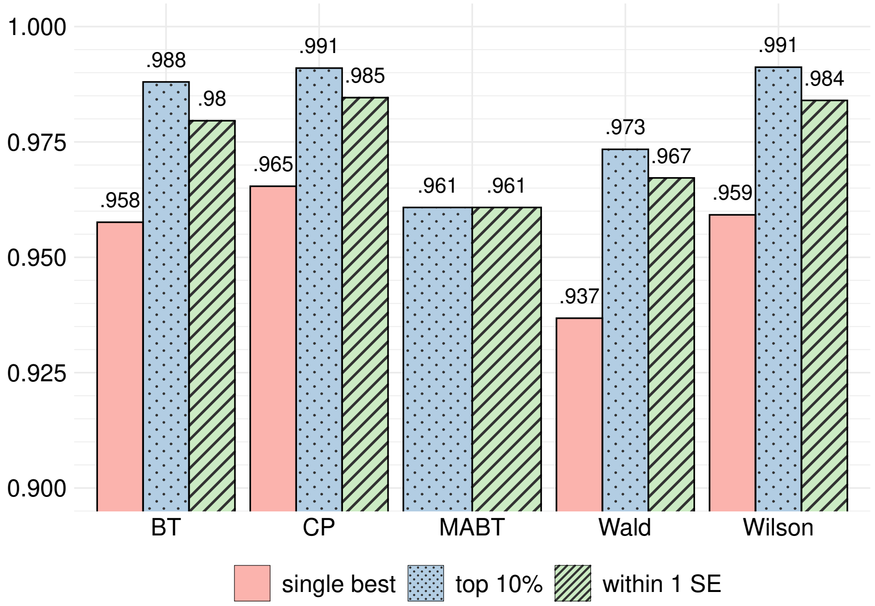


Figure 25: Observed coverage for prediction accuracy with case B features, learning sample size 300, evaluation sample size 100, and with cross-validation for validation performance estimation. Using the *single best* selection rule, Wald bounds are too liberal while BT, CP, and Wilson bounds as well as both types of MABT bounds are a bit conservative. All the Šidák-corrected bounds are even more conservative

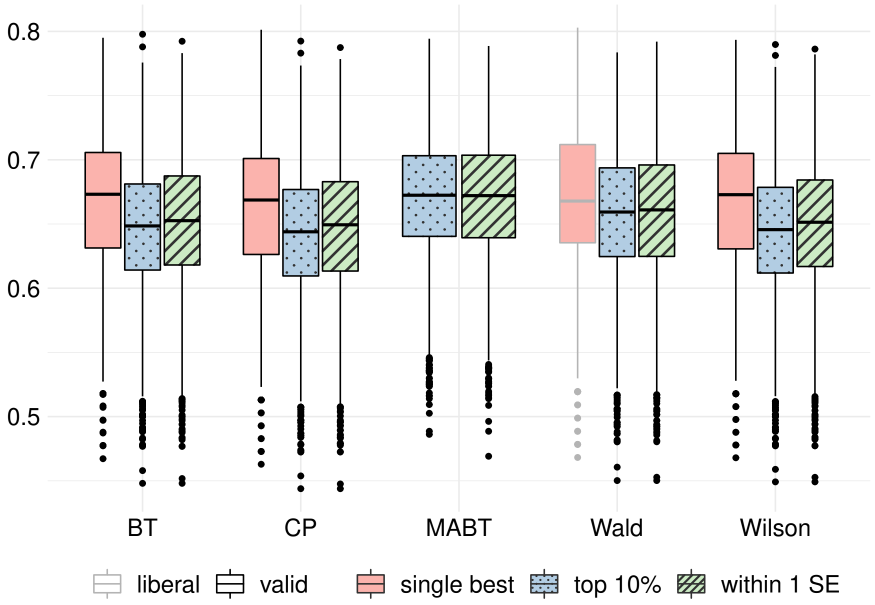


Figure 26: Lower confidence bounds for prediction accuracy with case B features, learning sample size 300, evaluation sample size 100, and with cross-validation for validation performance estimation. MABT bounds are largest, while the bounds from the *single best* selection rule are slighly smaller. The Šidák-corrected bounds are even smaller than those

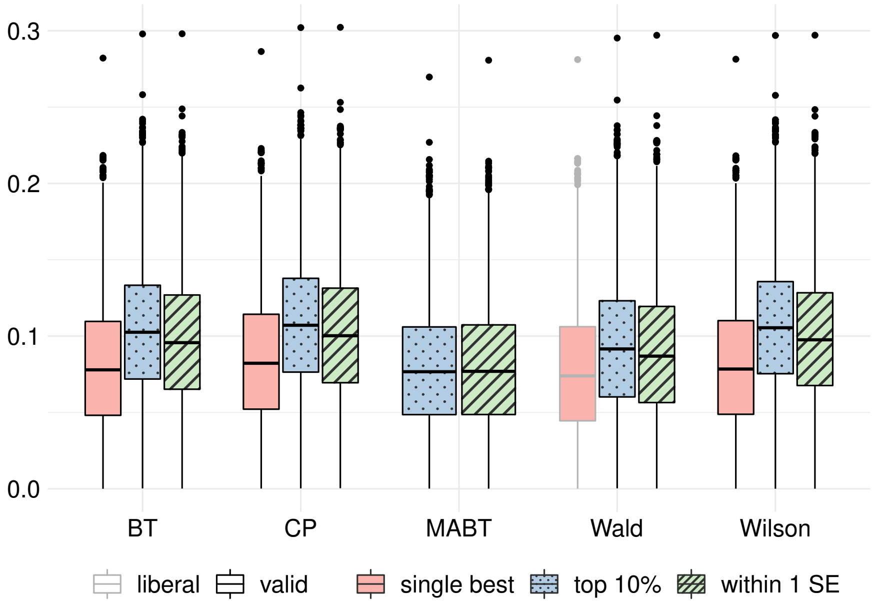


Figure 27: Tightness for prediction accuracy with case B features, learning sample size 300, evaluation sample size 100, and with cross-validation for validation performance estimation. Wald bounds are tightest, but they are too liberal. Among the valid bounds, MABT bounds are tightest, while the bounds from the *single best* selection rule are slightly less tight, and the Šidák-corrected bounds are even less tight than those

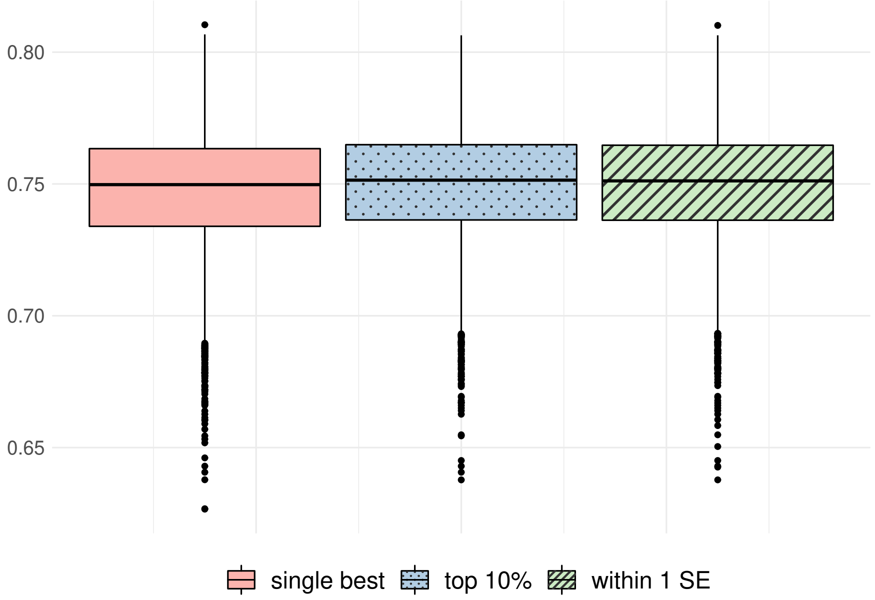


Figure 28: True prediction accuracy of the final selected model with case B features, learning sample size 300, evaluation sample size 100, and with cross-validation for validation performance estimation. The true prediction accuracies from the *top 10%* and *within 1 SE* selection rule are slightly higher than those from the *single best* selection rule

## 8 Prediction Accuracy, Case B Features, Sample Size 200, Without Cross-Validation

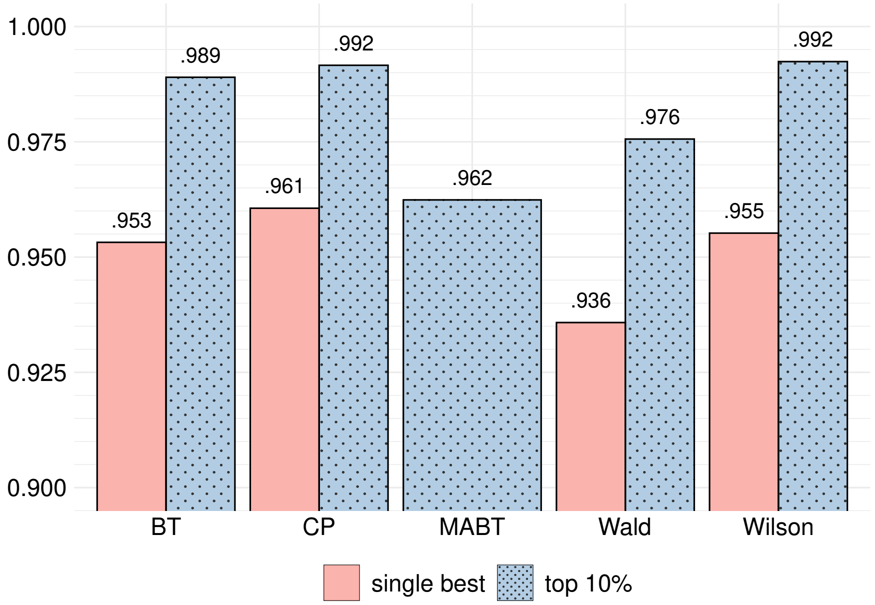


Figure 29: Observed coverage for prediction accuracy with case B features, learning sample size 300, evaluation sample size 100, and without cross-validation for validation performance estimation. Using the *single best* selection rule, Wald bounds are too liberal, while BT and Wilson bounds are slightly conservative, and CP bounds as well as MABT bounds are a bit more conservative. The Šidák-corrected bounds are very conservative

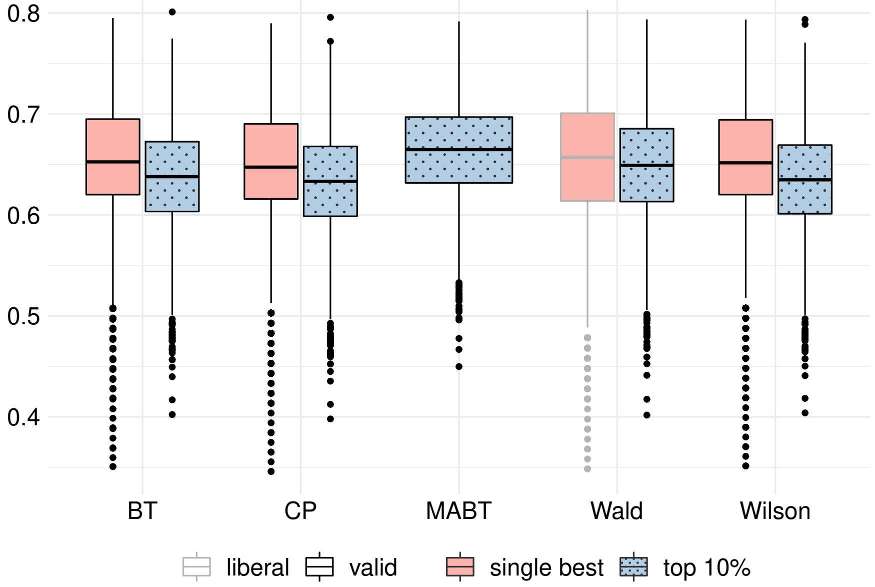


Figure 30: Lower confidence bounds for prediction accuracy with case B features, learning sample size 150, evaluation sample size 50, and without cross-validation for validation performance estimation. MABT bounds are largest, while the bounds from the *single best* selection rule are a bit smaller, and the Šidák-corrected bounds are even smaller than those

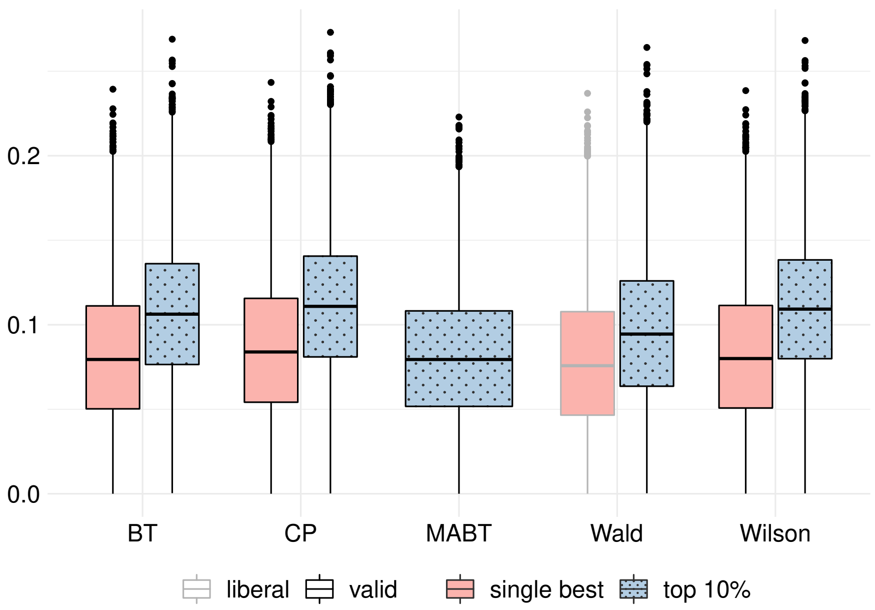


Figure 31: Tightness for prediction accuracy with case B features, learning sample size 150, evaluation sample size 50, and without cross-validation for validation performance estimation. Wald bounds are tightest, but they are too liberal. Among the valid bounds, MABT bounds are tightest. The bounds from the *single best* selection rule are only slightly less tight, and the Šidák-corrected bounds are visibly even less tight than those

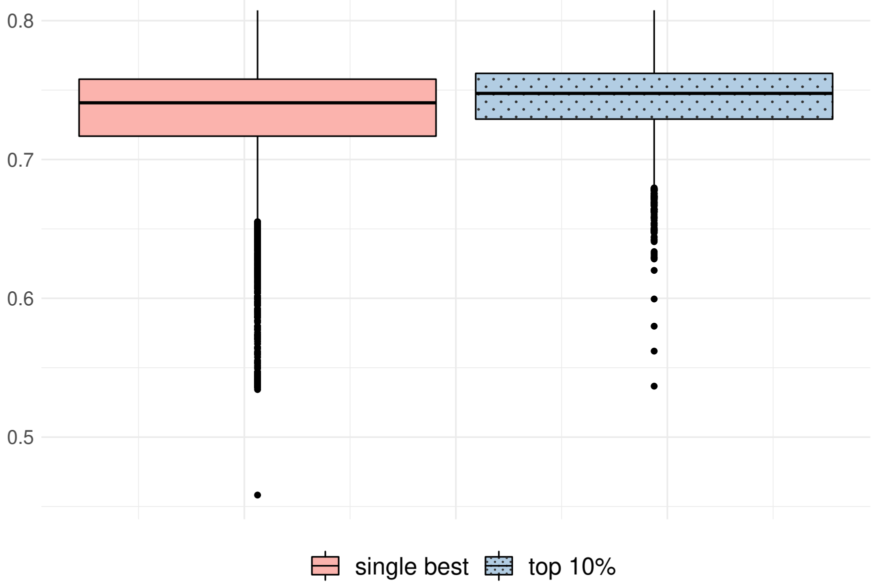


Figure 32: True prediction accuracy of the final selected model with case B features, learning sample size 150, evaluation sample size 50, and without cross-validation for validation performance estimation. The true prediction accuracies from the *top 10%* selection rule are slightly higher than from the *single best* selection rule

# 9 AUC, Case A Features, Sample Size 400, With Cross-Validation

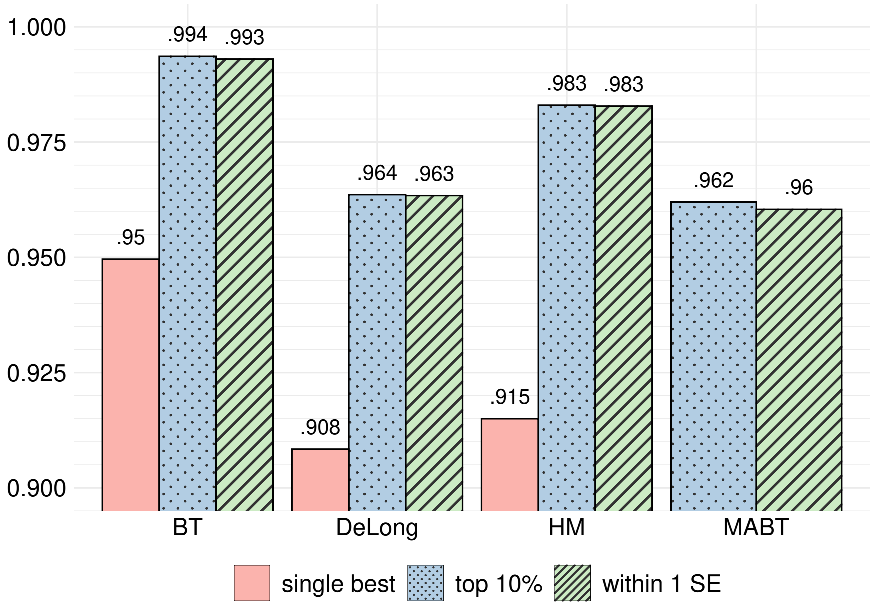


Figure 33: Observed coverage for AUC with case A features, learning sample size 300, evaluation sample size 100, and with cross-validation for validation performance estimation. Using the *single best* selection rule, BT bounds have the nominal level, while DeLong an HM bounds are very liberal. The MABT bounds as well as the Šidák-corrected DeLong bounds are conservative, while the remaining Šidák-corrected bounds are heavily conservative

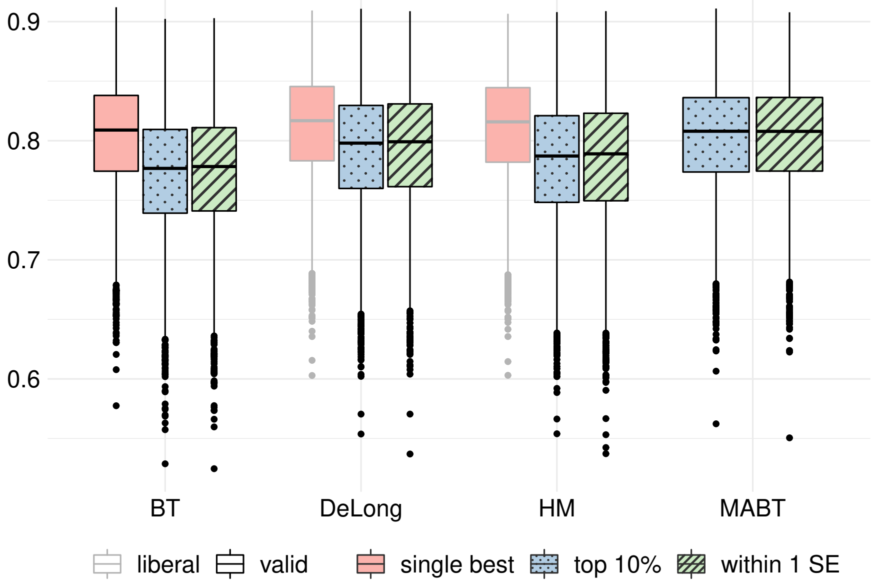


Figure 34: Lower confidence bounds for AUC with case A features, learning sample size 300, evaluation sample size 100, and with cross-validation for validation performance estimation. Using the *single best* selection rule, DeLong and HM bounds are largest, but they are both very liberal. MABT bounds and BT bounds from the *single best* selection rule are largest. The Šidák-corrected bounds are all clearly smaller

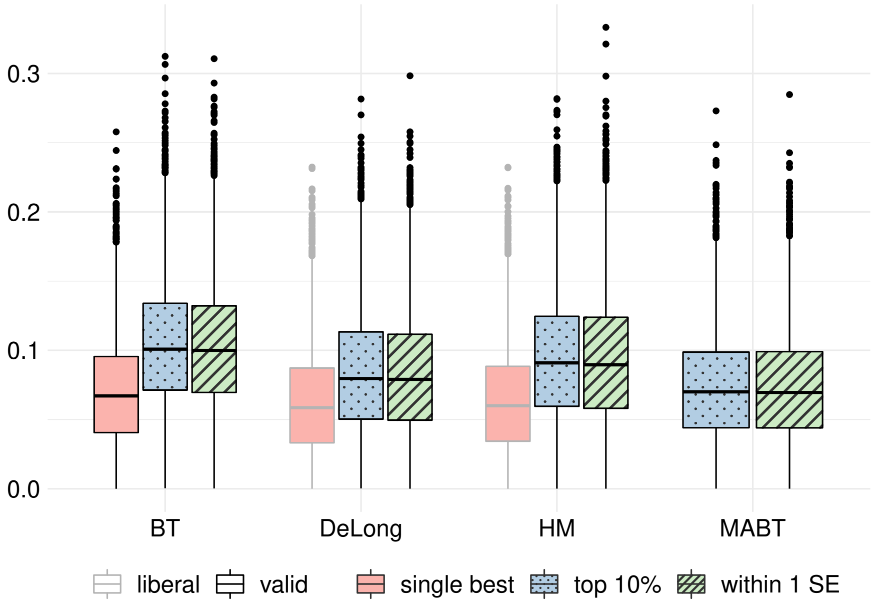


Figure 35: Tightness for AUC with case A features, learning sample size 300, evaluation sample size 100, and with cross-validation for validation performance estimation. Using the *single best* selection rule, DeLong and HM bounds are tightest, but they are both very liberal. Among the valid bounds, BT bounds from the *single best* selection rule as well as MABT bounds are tightest. The Šidák-corrected bounds are less tight

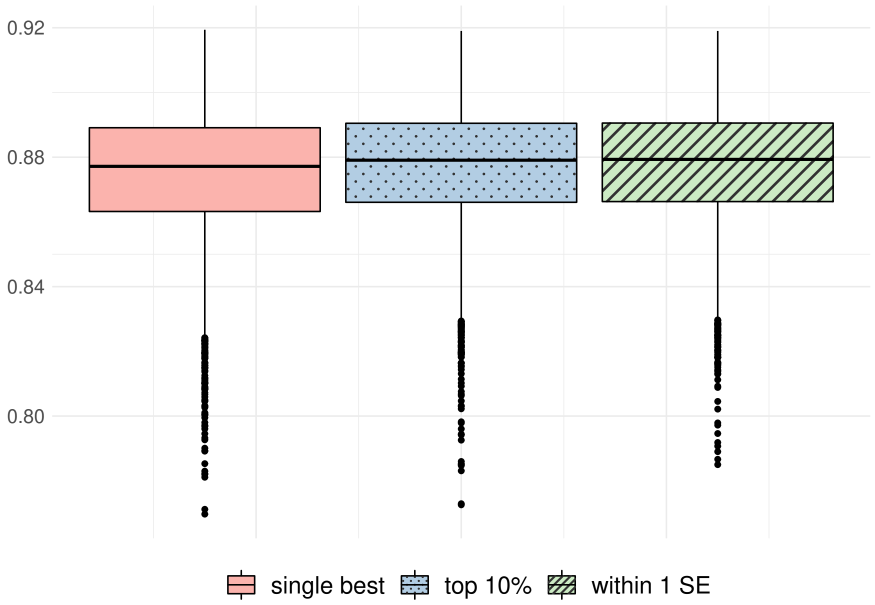


Figure 36: True AUC of the final selected model with case A features, learning sample size 300, evaluation sample size 100, and with cross-validation for validation performance estimation. The true AUCs from the *top 10%* and *within 1 SE* are slightly higher than those from the *single best* selection rule

## 10 AUC, Case A Features, Sample Size 600, With Cross-Validation

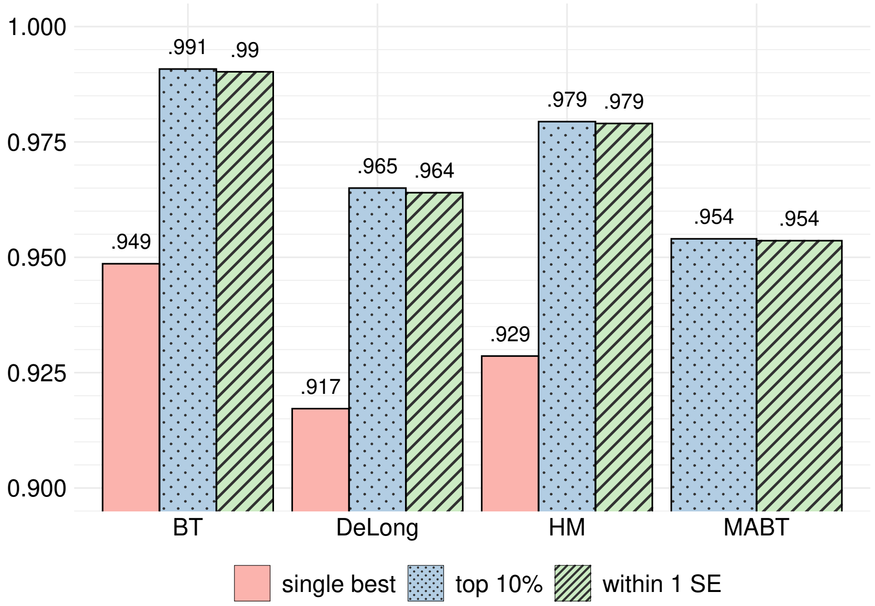


Figure 37: Observed coverage for AUC with case A features, learning sample size 450, evaluation sample size 150, and with cross-validation for validation performance estimation. Using the *single best* selection rule, DeLong and HM bounds are very liberal, while BT bounds are very close to the nominal level. MABT bounds are slightly conservative, and the Šidák-corrected bounds are very conservative

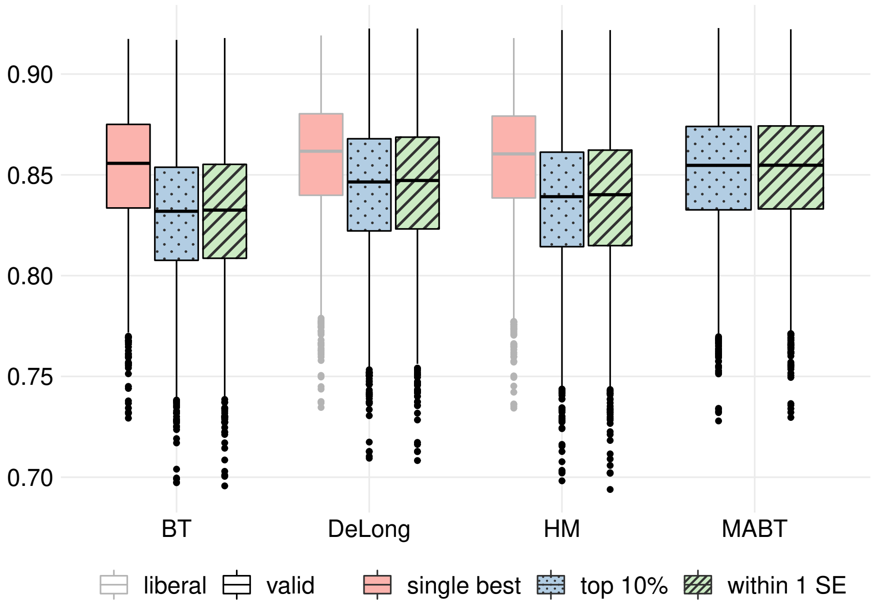


Figure 38: Lower confidence bounds for AUC with case A features, learning sample size 450, evaluation sample size 150, and with cross-validation for validation performance estimation. Using the *single best* selection rule, DeLong and HM bounds are largest, but they are both too liberal. BT bounds from the *single best* selection rule as well as MABT bounds are largest among the valid bounds. The Šidák-corrected bounds are all clearly smaller

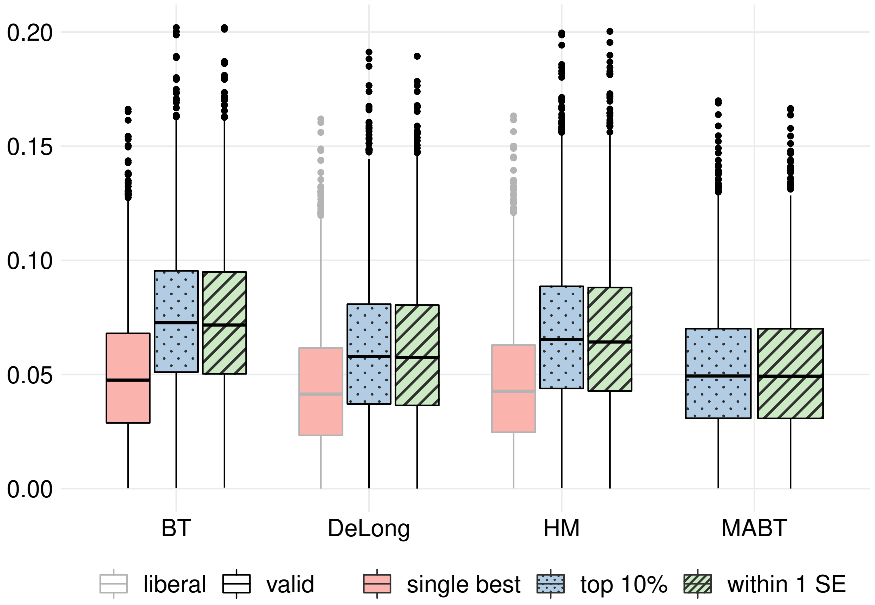


Figure 39: Tightness for AUC with case A features, learning sample size 450, evaluation sample size 150, and with cross-validation for validation performance estimation. Using the *single best* selection rule, DeLong and HM bounds are tightest, but they are both very liberal. Among the valid bounds, BT from the *single best* selection rule as well as MABT bounds are tightest. The Šidák-corrected bounds are clearly less tight

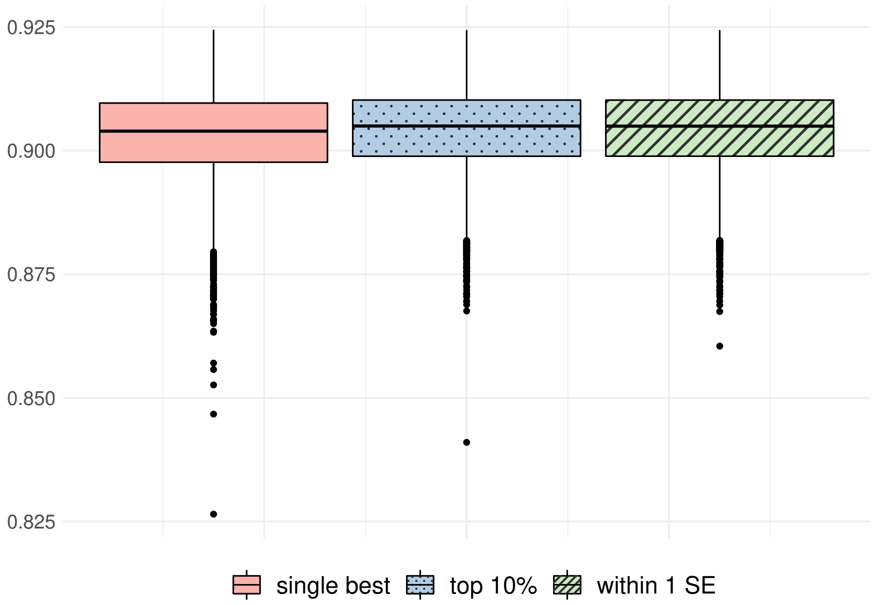


Figure 40: True AUC of the final selected model with case A features, learning sample size 450, evaluation sample size 150, and with cross-validation for validation performance estimation. True AUCs from the *top 10%* and the *within 1 SE* selection rule are both slightly higher than from the *single best* selection rule

## 11 AUC, Case B Features, Sample Size 400, With Cross-Validation

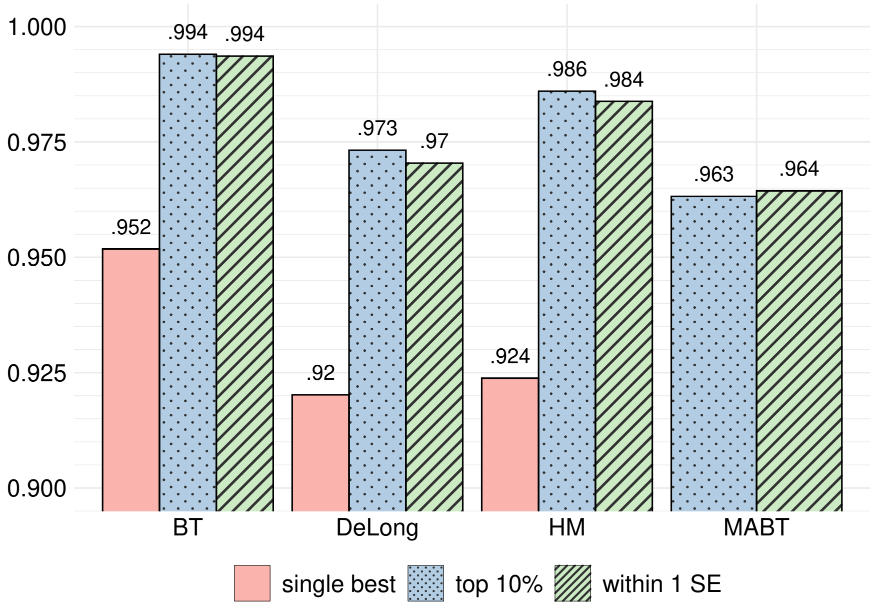


Figure 41: Observed coverage for AUC with case B features, learning sample size 300, evaluation sample size 100, and with cross-validation for validation performance estimation. Using the *single best* selection rule, DeLong and HM are very liberal, while BT bounds are very close to the nominal level. MABT bounds are conservative, and the Šidák-corrected bounds are strongly conservative

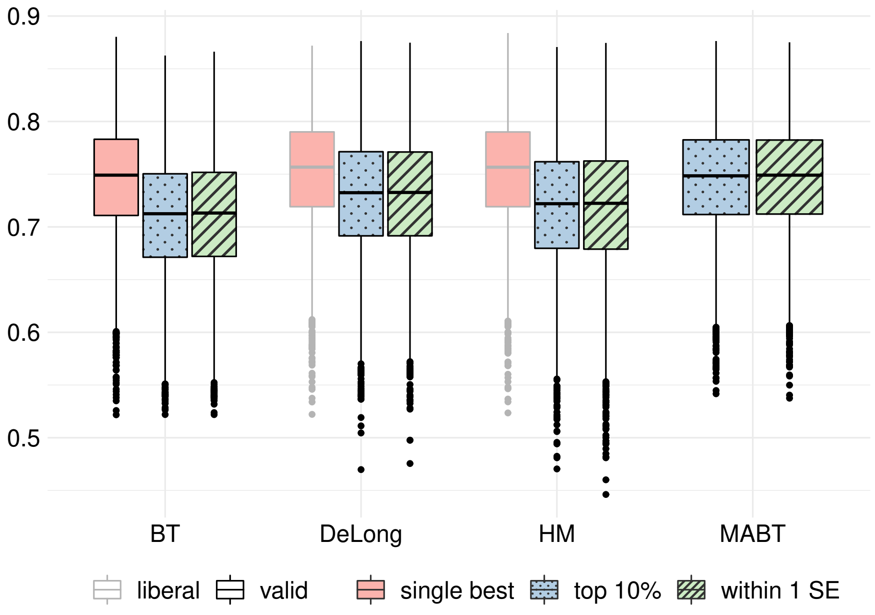


Figure 42: Lower confidence bounds for AUC with case B features, learning sample size 300, evaluation sample size 100, and with cross-validation for validation performance estimation. Using the *single best* selection rule, DeLong and HM bounds are largest, but they are both too liberal. Among the valid bounds, BT bounds from the *single best* selection rule as well as MABT bounds are largest. The Šidák-corrected bounds are clearly smaller

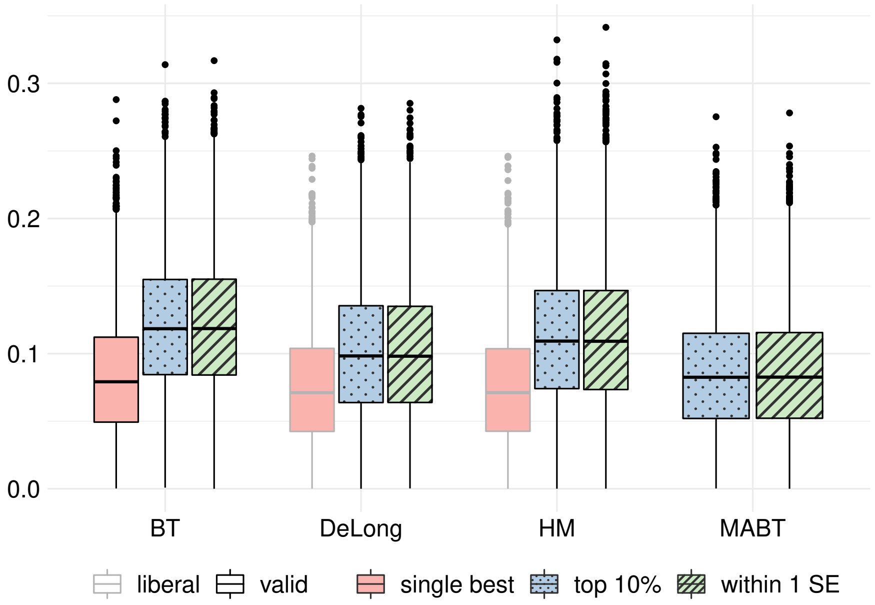


Figure 43: Tightness for AUC with case B features, learning sample size 300, evaluation sample size 100, and with cross-validation for validation performance estimation. Using the *single best* selection rule, DeLong and HM bonds are tightest, but they both are very liberal. Among the valid bounds, BT bounds from the *single best* selection rule as well as MABT bounds are tightest. The Šidák-corrected bounds are visibly less tight

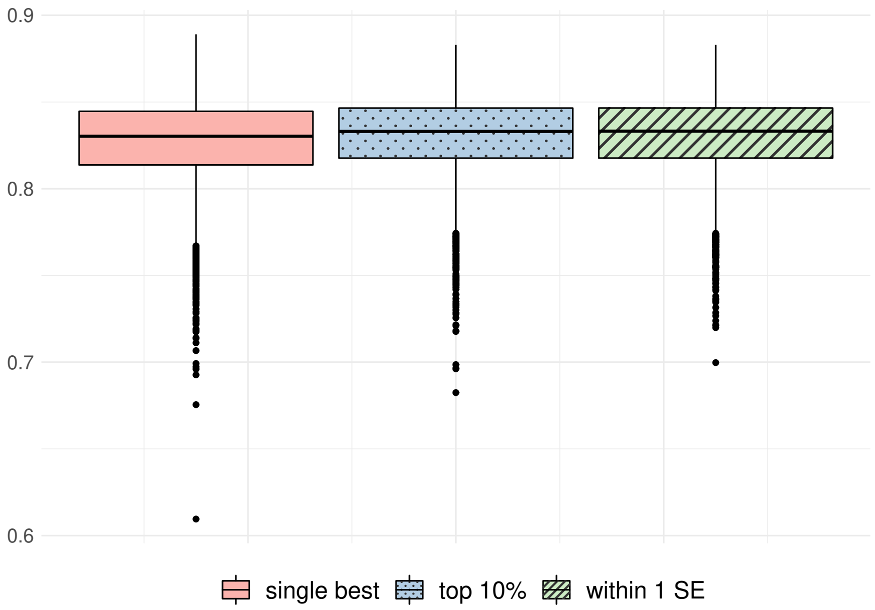


Figure 44: True AUC of the final selected model with case B features, learning sample size 300, evaluation sample size 100, and with cross-validation for validation performance estimation. The true AUCs from the *top 10%* and *within 1 SE* selection rule are slightly higher than those from the *single best* selection rule

## 12 AUC, Case B Features, Sample Size 600, With Cross-Validation

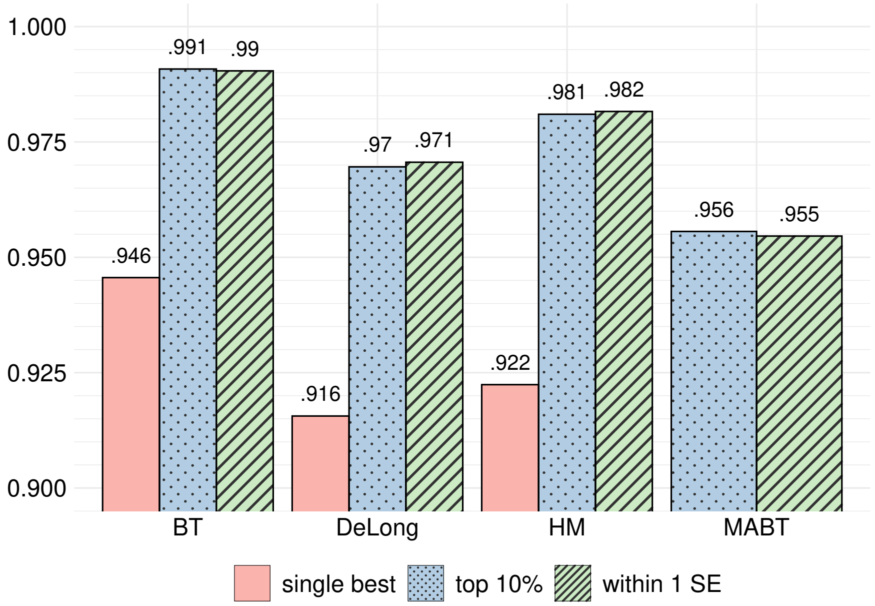


Figure 45: Observed coverage for AUC with case B features, learning sample size 450, evaluation sample size 150, and with cross-validation for validation performance estimation. Using the *single best* selection rule, DeLong and HM bounds are very liberal, while BT is only slightly liberal and close to the nominal level. MABT bounds are only slightly conservative, and the Šidák-corrected bounds are very conservative

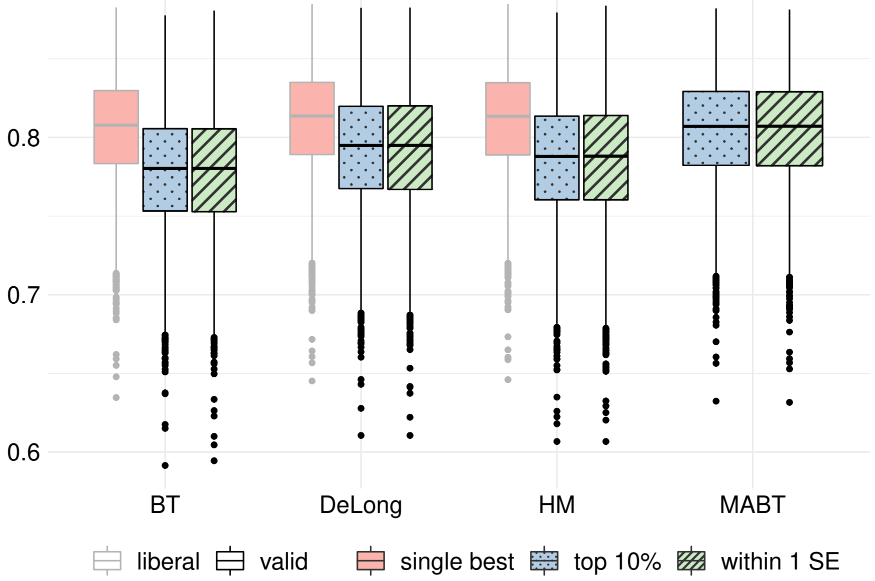


Figure 46: Lower confidence bounds for AUC with case B features, learning sample size 450, evaluation sample size 150, and with cross-validation for validation performance estimation. Using the *single best* selection rule, DeLong, HM, and BT bounds are largest, but they all are too liberal. Among the valid bounds, MABT bounds are largest, and the Šidák-corrected bounds are visibly smaller

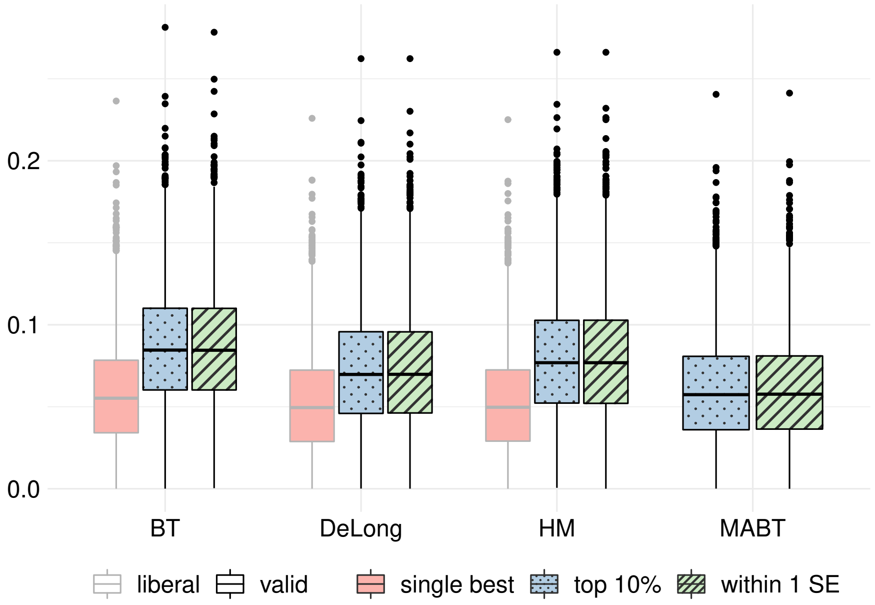


Figure 47: Tightness for AUC with case B features, learning sample size 450, evaluation sample size 150, and with cross-validation for validation performance estimation. Using the *single best* selection rule, DeLong, HM, and BT bounds are tightest, but they all are too liberal. Among the valid bounds, MABT bounds are tightest, while the Šidák-corrected bounds are visibly less tight

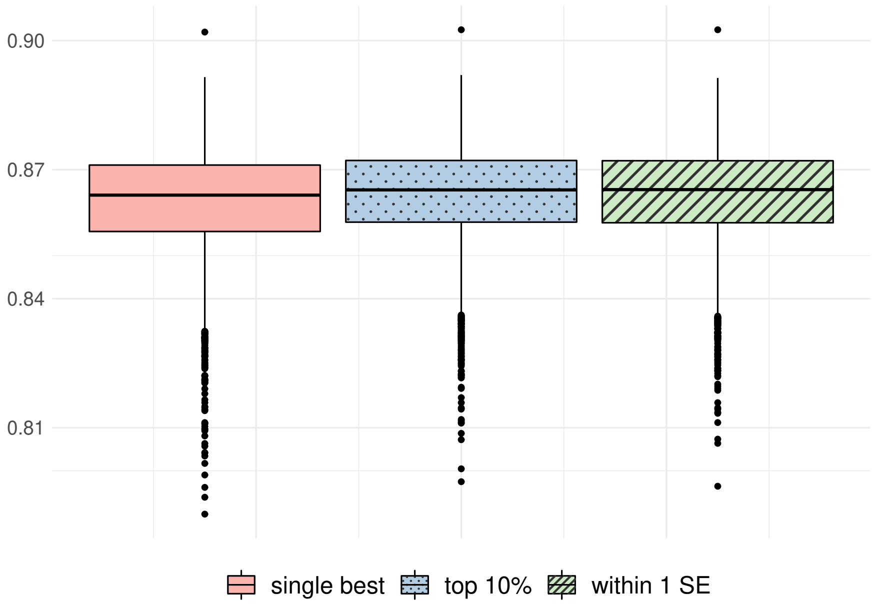


Figure 48: True AUC of the final selected model with case B features, learning sample size 450, evaluation sample size 150, and with cross-validation for validation performance estimation. The true AUCs from the *top 10%* and *within 1 SE* selection rules are slightly higher than those from the *single best* selection rule
